# Supplementary material for: ISO: Overlap of Computation and Communication within Seqenence For LLM Inference
Source: arXiv:2409.11155 source file (2024-09-04)
Supplement: Supplementary file 1 [file appendix.tex]

\newpage
\section{Appendix}
